# Supplementary material for: Many-body perturbation theory and non-perturbative approaches: the screened interaction as key ingredient
Source: arXiv:1710.06669 source file (2017-10-18)
Supplement: Supplementary file 1 [file appendix.tex]

\walter{To be written entirely. Below, some notes on the content.}

Here is the proof that for $C=0$ and $a=\y00{}^{-1}$ the function \eqref{opmansatz} goes to $y_0(x)$
when $v\to 0$.
